# Supplementary material for: How roughness and thermal properties of a solid substrate determine the Leidenfrost temperature: Experiments and a model
Source: arXiv:2305.13767 source file (2023-05-23)
Supplement: Supplementary file 1 [file SM.pdf]

# How roughness and thermal properties of a solid substrate determine the Leidenfrost temperature: Experiments and a model
# Supplementary materials

Yuki Wakata, Ning Zhu, Xiaoliang Chen, Sijia Lyu, Detlef Lohse,* Xing Chao,† and Chao Sun‡
(Dated: May 23, 2023)

## 1. EXPERIMENTAL METHODS AND MATERIALS

### 1.1 Measuring the Leidenfrost temperature

To obtain the Leidenfrost temperature under different conditions, we measure the lifetime of a sessile droplet, $\tau$, as a function of initial surface temperature $T_{s0}$. The experimental setup is shown in Fig.S1.

To get a constant surface temperature, temperature sensor #1 (Pt100, Twidec MT-6260HA) operates with four immersion heating rods (Twidec TC-R101A 10mm) to stabilize the temperature of the brass heating base through a PID controller (Honeywell DC1040), while temperature sensor #2 (Pt100, Twidec MT-2250A) placed 2mm under the surface measures the surface temperature of the test substrate. The test substrates are made of aluminum, brass, carbon steel (Type 1045) and stainless steel (Type 304). Table S1 lists the thermal properties of these materials. The different surface roughnesses of the substrates are artificially made by changing the size of the processing cutter. Table S2 lists the informations of all the test substrates used in our experiments.

Liquid droplets are generated by a syringe pump (Harvard Apparatus PHD ULTRA) with a 15-gauge stainless steel needle. Using a flow rate of 1.2 mL/min and an injecting time of 1.75 s, the initial volume of the droplet is controlled to be 30.6 µL. The volume of the droplet is obtained through measuring the total mass of ten droplets using an analysis balance (Meilen MCS220) and dividing the averaged mass of one droplet by liquid density at room temperature (25°C).

A high-speed camera (Photron Fastcam NOVA S12) with macro lens (Nikon 105 mm) is used to record the entire evaporation process. In our previous work [1], we analyzed the images taken by the high-speed camera to obtain the drop volume. In the present work, the obtained volume is only used to observe the evaporation process. The lifetime $\tau$ of the drop is counted from the deposited time till total evaporation or take off (final fate of a Leidenfrost drop [2]). For each surface temperature, the corresponding lifetime of the droplet is measured over three times. According to Ref. [3], the surface temperature that relates to the longest lifetime on superheated surfaces is defined as the Leidenfrost temperature. Our experiments use the same criterion to determine the Leidenfrost temperature. The influences of thermal diffusivity and surface roughness on the Leidenfrost temperature is shown in Fig. 2c in the main Letter.

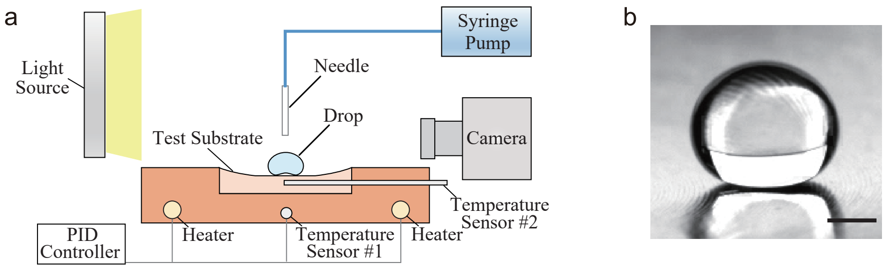


FIG. S1: **a.**The schematic of the experimental setup for measuring the Leidenfrost temperature. **b.**Side view of a Leidenfrost droplet on an aluminum surface with surface roughness $S_a = 1.0$ µm. The scale bar represents 1 mm.

### 1.2 Illustrating the surface cooling using infrared camera

To illustrate the surface cooling caused by a Leidenfrost droplet, the experimental setup in Fig. 1a in the main Letter is used. The temperature sensors, heating base, heaters, syringe pump and the needle are the same as the setup

TABLE S1: Thermal properties of the selected materials

| Properties | Units | Aluminum (Al) | Brass (Br) | Carbon Steel Type 1045 (CS) | Stainless Steel SUS304 (SS) |
|---|---|---|---|---|---|
| Thermal conductivity $k_s$ | W/m K | 220 | 119 | 51.9 | 16.3 |
| Density $\rho_s$ | kg/m$^3$ | 2707 | 8800 | 7870 | 7817 |
| Specific heat $c_s$ | J/kg K | 896 | 380 | 486 | 460 |
| Thermal diffusivity $\alpha = k_s/\rho_s c_s$ | m$^2$/s | 0.907 $\times 10^{-4}$ | 0.356 $\times 10^{-4}$ | 0.136 $\times 10^{-4}$ | 0.045 $\times 10^{-4}$ |

TABLE S2: Information of the test substrates

| Substrate Number | Material | Thermal diffusivity $\alpha$ ($\times 10^{-4}$m$^2$/s) | Surface roughness $S_a$ (µm) |
|---|---|---|---|
| 1 | Aluminum | 9.07 | 1.0 |
| 2 | Aluminum | 9.07 | 1.7 |
| 3 | Brass | 3.56 | 0.6 |
| 4 | Brass | 3.56 | 1.8 |
| 5 | Brass | 3.56 | 2.7 |
| 6 | Carbon Steel | 1.36 | 0.1 |
| 7 | Carbon Steel | 1.36 | 0.6 |
| 8 | Carbon Steel | 1.36 | 1.8 |
| 9 | Stainless Steel | 0.45 | 0.5 |
| 10 | Stainless Steel | 0.45 | 1.4 |
| 11 | Stainless Steel | 0.45 | 2.5 |

in Section 1.1. In the experiment, we place a water drop on a superheated substrate and use a needle to control the movement of the droplet. The droplet evaporates at a fixed location for 60 s, then it is removed by the needle within 0.05 s, exposing the surface underneath (see Movie S1). After that, the temperature field of the solid surface from top view is measured using an infrared camera (TELOPS FAST L200) with a reflecting mirror (HengYangGuangXue GMH12-025-AG). The emissivity of the surface is determined by the temperature measured by the temperature sensor #2.

## 2. THEORETICAL MODEL AND CALCULATION METHODS

We develop a theoretical model that focuses on the evaporation process of a Leidenfrost droplet from a certain volume to complete evaporation (see Fig. 3a in the main Letter). The temperature variation of the substrate during the evaporation process is considered. The evaporation process is assumed to be quasi-static, which is justified as the time scale of droplet evaporation is the largest comparing with thermal and viscous relaxation times [4]. The internal flow and the temperature gradient in the drop is neglected.

The model consists of two parts - theoretical definition of the drop shape and calculation of the surface temperature field, and will be introduced in the following two subsections.

### 2.1 Theoretical definition of the drop shape

For theoretical determination of the drop shape, the drop surface is divided into upper and lower regions by the patch point (see Fig. S2) [4]. The shape of the upper surface is governed by a balance between the hydro-static pressure and the surface tension through the equation

$$\sigma\kappa(z) - \rho_l g(z - z_{\text{top}}) = \sigma\kappa_{\text{top}},$$

where $\sigma$ is the surface tension of the liquid, $\kappa(z)$ is the local curvature at the drop surface, $\rho_l$ the liquid density, and $z$ the vertical coordinate. The subscript 'top' refers to values at the crest of the drop. With a given $\kappa_{\text{top}}$, the upper profile of the drop is calculated till the patch point.

For the surface below the patch point, the pressure of the vapor layer $P_g$ is taken into consideration, yielding $P_\mathrm{g} = P_0 - \rho_l g\delta + \sigma\kappa$, where $P_0$ is the environmental pressure and $\delta$ the vapor film thickness. Because of the small thickness of the vapor layer, the lubrication approximation is implemented to simplify the momentum equation [3], leading to

$$\frac{\mathrm{d}^2 u}{\mathrm{d}z^2} = \frac{1}{\mu_g}\frac{\mathrm{d}P_g}{\mathrm{d}r},$$

where $u$ is the vapor velocity in horizontal direction and $\mu_g$ the dynamic viscosity of the vapor. The continuity equation in the vapor layer can be formulated as

$$\frac{1}{r}\frac{\partial(ru)}{\partial r} + \frac{\partial w}{\partial z} = 0,$$

where $w$ is the velocity in the z-direction and corresponds to the volume flux of evaporation from the lower surface of the drop. The vapor velocity at the drop interface $w\big|_{z=\delta}$ is obtained by the energy equation

$$\rho_g(-w\big|_{z=\delta})L = k_g\frac{T_\mathrm{s} - T_\mathrm{sat}}{\delta},$$

where $\rho_g$ is the gas density, $L$ is the latent heat of the liquid, $k_g$ the thermal conductivity of the gas, $T_\mathrm{s}$ the surface temperature and $T_\mathrm{sat}$ the saturation temperature of the liquid. Integrating the momentum and the continuity equation, differential equations of film thickness $\delta(r)$ are obtained and solved by combining the boundary conditions at the symmetrical axis and at the patch point (see (18)-(20) in Ref. [5]). Combining the upper and lower parts of the droplet shape gives the overall geometry, and the volume of the drop can be obtained through integration in cylindrical coordinates.

Note that the volume $V$ of the droplet is fully determined by curvature $\kappa_\mathrm{top}$ (defines the drop geometry) and surface temperature $T_\mathrm{s}$. Therefore, on a surface with a certain $T_\mathrm{s}$, we can obtain a one-to-one correspondence between $V$ and $\kappa_\mathrm{top}$. Here we calculate the $V(\kappa_\mathrm{top})$ dependence of water droplets on surfaces with $T_\mathrm{s} = 160 \sim 360°\mathrm{C}$ and of ethanol droplets on surfaces with $T_\mathrm{s} = 120 \sim 280°\mathrm{C}$. The interval of the calculating surface temperature is 5°C.

### 2.2 Evaporation rate of the Leidenfrost drop

The volume evaporation rate $\mathrm{d}V/\mathrm{d}t$ of the current time step is calculated through integrating the evaporation flux [5]. For the upper surface, the evaporation flux is assumed to follow the steady diffusion equation $\frac{1}{r_s^2}\frac{d}{dr_s}\left(r_s^2\frac{dc}{dr_s}\right) = 0$, where $c$ is the radial coordinate in the spherical coordinate system and $c$ the molar concentration of the vapor in the gas phase.

For the lower surface, the evaporation flux is calculated through the energy equation $\rho_g(-w\big|_{z=\delta})L = k_g\frac{T_\mathrm{s}-T_\mathrm{sat}}{\delta}$ listed before. The volume for the next time step is then obtained through $V(\mathrm{i}+1) = V(\mathrm{i}) + \frac{\mathrm{d}V}{\mathrm{d}t}\mathrm{d}t$.

### 2.3 Calculation of the surface temperature field.

The variation of the temperature profile of the solid substrate $T(r,z)$ during the evaporation process is numerically calculated using the transient heat diffusion equation:

$$\frac{1}{\alpha}\frac{\partial T}{\partial t} = \frac{\partial}{\partial r}\left(r\frac{\partial T}{\partial r}\right) + \frac{\partial^2 T}{\partial z^2}.$$

As shown in Fig. S2, we divide the substrate into two regions according to the projected area of the lower drop surface. We assume that the cooling heat flux $q$ only affects the region right beneath the lower droplet surface ($r < R_\mathrm{p}$), while an adiabatic boundary condition is used for outer region ($r > R_\mathrm{p}$). The cooling heat flux $q$ on the solid surface is obtained through the equation: $q(r) = -\frac{k_\mathrm{g}}{\delta(r)}(T_\mathrm{s} - T_\mathrm{sat})$. The bottom and the side boundaries of the solid substrate is assumed to have constant temperature equal to the initial temperature of the substrate $T_0$. Averaging the surface temperature right beneath the lower droplet surface $T(r < R_\mathrm{p}, z = 0)$, we get the surface temperature $T_s$ for calculating the drop shape for the next time step. We use implicit methods to calculate the time differencing schemes of the transient heat diffusion equation.

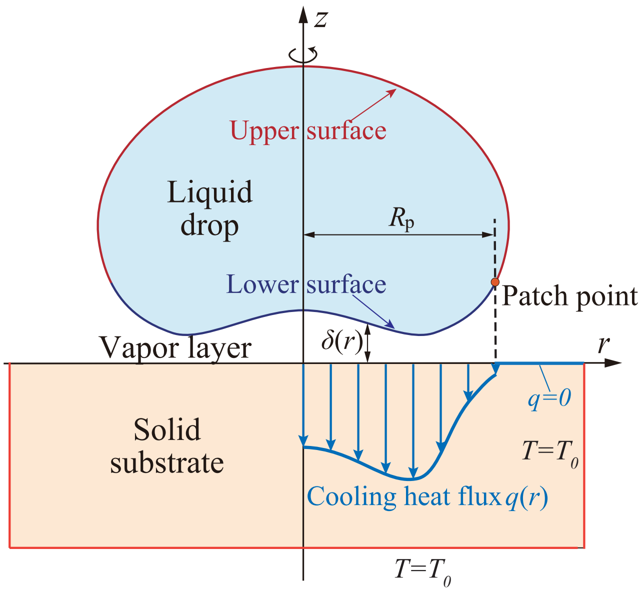


FIG. S2: The schematic of the theoretical model.

### 2.4 Calculation procedure of the evaporation process

In the $i$th time step, the surface temperature changes from $T_s(i)$ to $T_s(i+1)$, where $T_s(i+1)$ is an also unknown variable. We use the average surface temperature $T_s^* = \frac{T_s(i)+T_s(i+1)}{2}$ in the time step for defining the drop geometry through the $V - \kappa_{top}$ dependence (see Section 2.1). After the film geometry is obtained, the cooling heat flux and the variation of the temperature field of the solid substrate can be calculated using the method described in Section 2.2. Then the surface temperature at the end of the time step $T_s(i+1)$ is calculated.

Iterative methods are use throughout the procedure to get the value of $T_s^*$. We first assume a $T_s^*$ to calculate the $T_s(i+1)$ through the procedure described before, then compare the average value of $T_s(i)$ and $T_s(i+1)$ with the assumed $T_s^*$. The new assumption value of $T_s^*$ is obtained as $\omega$ times the deviation value, where $\omega$ is an input iteration factor and is set to 0.2 in our calculations.

We calculate the evaporation process of a Leidenfrost drop with the initial volume of $V_0 = 30.6$ µL till a very small volume of $V_{end} = 0.4$ µL. Near and below $V_{end}$, the lubrication approximation is no longer valid [2]. For 2D transient heat transfer calculation, the width and the height of the grid, $\Delta x$ and $\Delta y$, are both set as $2 \times 10^{-5}$ m. The time step $\Delta t$ is calculated using the function $\Delta t = Fo(\Delta x \Delta y)/\alpha$, where Fourier number $Fo$ is set as 20 and $\alpha$ is the thermal diffusivity of the substrate material. The whole program is run on a personal computer using MATLAB software. The real calculation time is about 10 hours for one $\delta_c(T_{s0})$ dependency curve of a particular material in Fig. 4b in the main Letter. Combining the $\delta_c(T_{s0})$ curve with the function $\delta_c = \delta_c^* + S_a$, we are able to predict the Leidenfrost temperature on a certain surface.

## 3. FILM THICKNESS OF SMALL LEIDENFROST DROPS

About the film thickness of very small drops, it is observed in former experiments [2] that with the shrinkage of the drop, the film thickness will decrease to a minimum value , then will increase dramatically. Our model also qualitatively captured this phenomenon, which can be seen in Figure S3. However, as the lubrication approximation is no longer valid when the film thickness is comparable to the drop radius, the model-calculated thickness is not accurate. Therefore, the final stage of the drop is not included in the results.

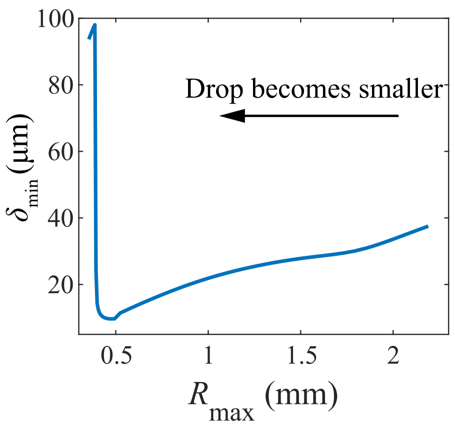


FIG. S3: Minimal film thickness versus drop radius at surface temperature $T_{s0} = 300°C$

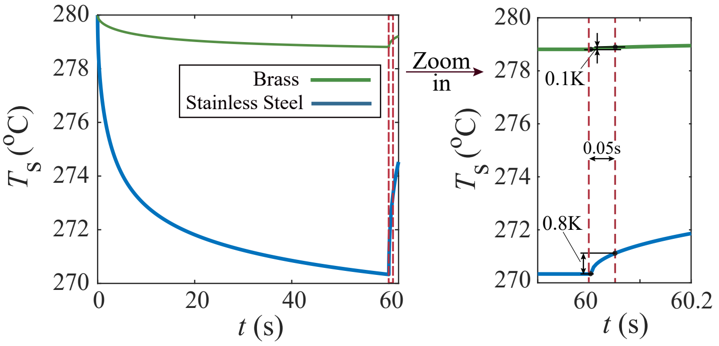


FIG. S4: Variation of surface temperature with time in the cooling-recovering process through model calculation.

## 4. TEMPERATURE VARIATION DURING THE INFRARED EXPERIMENT

In order to demonstrate that the method introduced in Section 1.2 yields accurate information about the surface temperature field, we need to ensure two issues. One is that the droplet has little cooling effect on the surface temperature in the moving path. Another is that the recovery of the surface temperature is negligible during the time when the droplet moves away and the solid surface is exposed to infrared camera (about 0.05 s).

To study these two issues, we slightly modified the calculation model introduced in the main Letter. In the calculation, we let a droplet evaporate with a constant radius $R \approx 2$ mm on brass and stainless steel surfaces. The surfaces are cooled for 60 seconds, following the transient heat diffusion equation $\frac{1}{\alpha}\frac{\partial T}{\partial t} = \frac{\partial}{\partial r}\left(r\frac{\partial T}{\partial r}\right) + \frac{\partial^2 T}{\partial z^2}$. Then, the cooling boundary condition is replaced by an adiabatic boundary condition, which corresponds to the condition that the surface temperature recovers after the drop is removed.

Fig.S2 shows the temperature variation during the cooling and the recovering process. The surface temperature of the stainless steel is reduced by 9 K after 60 s, a value similar to that measured by the infrared camera (about 6 K, see Fig. 1c in the main Letter). Therefore, the accuracy of the theoretical calculation is confirmed. In the experiments, the residence time of the droplet in the moving path is about 0.05 s. In this time period, the surface temperature reduction is less than 0.2 K, which indicates that the droplet has less influence on the solid surface temperature field during its movement. About the recovery of the surface temperature, Fig.S2 shows the temperature variation during the cooling and the recovering process. The surface temperature increases 0.8 K and 0.1 K for stainless steel and brass surface during the time from the start of the removal of the drop to the moment when the solid surface can be photographed (from $t = 60$ s to $t = 60.05$ s). The temperature recovery is less than $1/10$ of the reduction during the cooling process. Therefore, it can be concluded that the current experimental method is applicable to demonstrate the temperature field of the solid surface.

* Electronic address: d.lohse@utwente.nl
† Electronic address: chaox6@tsinghua.edu.cn
‡ Electronic address: chaosun@tsinghua.edu.cn

[1] S. Lyu, H. Tan, Y. Wakata, X. Yang, C. K. Law, D. Lohse, and C. Sun, *On explosive boiling of a multicomponent Leidenfrost drop*, Proc. Natl. Acad. Sci. U. S. A. **118**, e2016107118 (2021).

[2] F. Celestini, T. Frisch, and Y. Pomeau, *Take off of small Leidenfrost droplets*, Phys. Rev. Lett. **109**, 034501 (2012).

[3] A.-L. Biance, C. Clanet, and D. Quéré, *Leidenfrost drops*, Phys. Fluids **15**, 1632 (2003).

[4] B. Sobac, A. Rednikov, S. Dorbolo, and P. Colinet, *Leidenfrost effect: Accurate drop shape modeling and refined scaling laws*, Phys. Rev. E **90**, 053011 (2014).

[5] C. Cai, I. Mudawar, H. Liu, and C. Si, *Theoretical Leidenfrost point (LFP) model for sessile droplet*, International Journal of Heat and Mass Transfer **146**, 118802 (2020).
